# Supplementary material for: Metal-insulator transition and topological properties of pyrochlore iridates
Source: arXiv:1505.01203 ancillary file (2015-05-05)
Supplement: Supplementary file 1 [file Pyrochlore_suppmat.pdf]

# Supplemental Material for
# "Metal-insulator transition and topological properties of pyrochlore iridates"

Hongbin Zhang,* Kristjan Haule, and David Vanderbilt
*Department of Physics and Astronomy, Rutgers University, Piscataway, USA*

In this Supplement we expand on the computational details and provide additional results concerning the spectral functions, entropies, structural information, and the evolution of the $X$-point eigenvalues with mixing fraction of the DMFT self-energy.

## I. COMPUTATIONAL DETAILS

Our charge self-consistent density functional theory (DFT) with dynamical mean-field theory (DMFT) calculations are done using the projection/embedding implementation[1] based on the WIEN2k package.[2] The auxiliary impurity problem is solved using the continuous-time quantum Monte Carlo method,[3] where a proper local basis adapted to the $IrO_6$ octahedra are chosen to minimize the sign problem. The exchange-correlation potential is approximated using the Perdew-Wang LDA functionals.[4] A set of system-independent local Coulomb interaction parameters $U = 4.5\,\mathrm{eV}$ and $J = 0.8\,\mathrm{eV}$ is used, which is determined to be good for Ruddlesden-Popper iridates.[5] The reason for using a larger $U$ compared to the typical value in LDA+U calculations is that the hybridizations and self-energies are computed in a large energy window of $\pm 10\,\mathrm{eV}$ around the Fermi energy ($E_\mathrm{F}$) in our DFT+DMFT calculations. We note that the 4f-electrons (when present) are treated using the open-core approximation, which is justified because the magnetic $4f$ moments become ordered at a temperature much lower than the typical metal-insulator transition temperature in the pyrochlore iridates (see for instance Ref. 6). The AIAO magnetic configuration is considered by transforming the local self-energies with site-dependent spin quantization axis to the global frame using proper Wigner rotations.[5] The free energies are evaluated following the methodology presented in Ref. 7. All calculations are carried out at the experimental lattice parameters.[8–12]

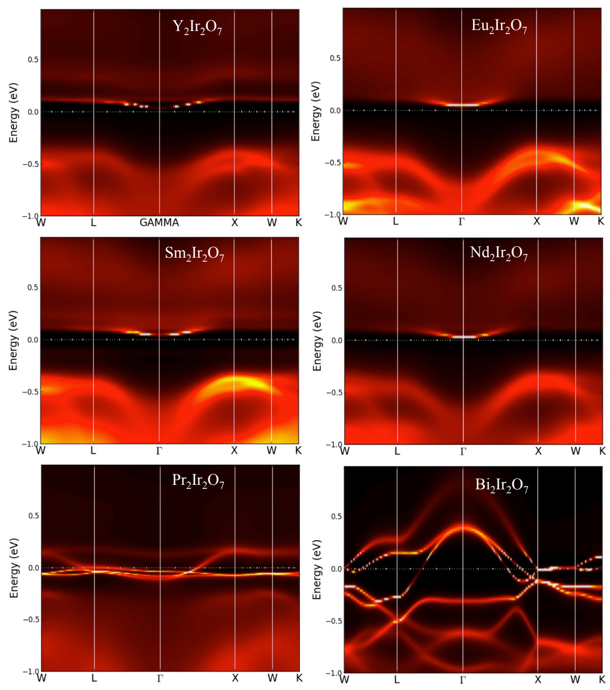


FIG. 1: (Color online) Spectral functions of six pyrochlore compounds $R_2Ir_2O_7$ (R=Y, Eu, Sm, Nd, Pr, and Bi) studied in this work. The spectral functions are shown for those compounds at corresponding ground states, that is, all-in-all-out magnetic insulating state for the Y, Eu, Sm, and Nd cases, and paramagnetic metallic state for the Pr and Bi compounds. Dashed white horizontal lines denote the Fermi energy.

The LDA+DMFT spectral functions for all six compounds are shown in Fig. 1. For the Y, Eu, Sm, and Nd compounds, the ground state is an all-in-all-out (AIAO) magnetic insulating state, with an average band gap of 0.3 eV, while both the Pr and Bi compounds are paramagnetic metals. Following Ref. 7, the free energies shown in Fig. 1 of the main text are obtained by evaluating the Luttinger-Ward functional using the self-consistent LDA+DMFT Green's functions. As given by Eq. 4 of Ref. 7, an accurate evaluation of the free energy of the LDA+DMFT quantum impurity model $F_\mathrm{imp} = E_\mathrm{imp} - TS_\mathrm{imp}$ is required, where $E_\mathrm{imp}$ ($S_\mathrm{imp}$) denotes the internal energy (entropy) of the corresponding impurity model. In Fig. 2, $S_\mathrm{imp}$ for $Nd_2Ir_2O_7$ in both the AIAO and PM states are shown, and the difference at 50 K is about 0.033 $k_B$ per Ir atom. Thus, it is justified to neglect the $TS_\mathrm{imp}$ contribution to the total free energies and their difference for the paramagnetic and AIAO magnetic states.

## II. STRUCTURAL ANALYSIS

For pyrochlore iridates, there are two distinct Wyckoff positions for oxygen atoms: 48f($x, \frac{1}{8}, \frac{1}{8}$) and 8b($\frac{3}{8}, \frac{3}{8}, \frac{3}{8}$). The oxygen atoms occupying the 48f position form the $IrO_6$ octahedra, hence the Ir-O bond length and the Ir-O-Ir bond angle (Fig. 3) are determined by a single parameter $x$. The variation of the $t_{2g}$ band-width and the averaged hybridization function are replotted in Fig. 3 together with the Ir-O bond length and the Ir-O-Ir bond angle, showing a strong correlation between the former two quantities with the latter two parameters. It is observed that the Bi compound is different from the other five

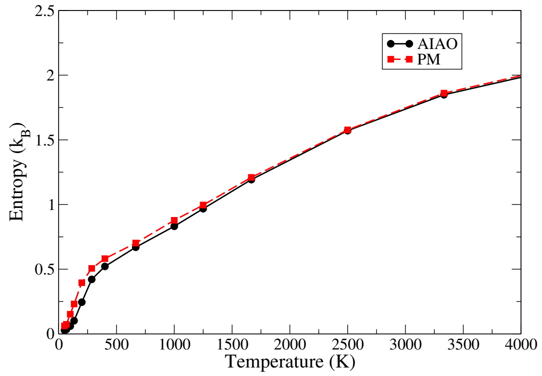


FIG. 2: (Color online) Entropy of the LDA+DMFT quantum impurity model for $Nd_2Ir_2O_7$ in the all-in-all-out (AIAO) magnetic state and in the paramagnetic (PM) state. Lines are guides for the eyes.

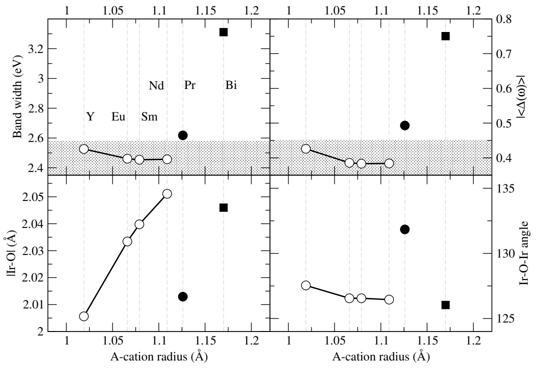


FIG. 3: (Color online) Variation of the (a) $t_{2g}$ bandwidth and (b) averaged hybridization function replotted together with (c) Ir-O bond length and (d) Ir-O-Ir bond angle with respect to the A-cation radius for the pyrochlore iridates studied in this work. Hollow (solid) symbols indicate that the corresponding ground state is insulating (metallic). Lines are guides for the eyes.

compounds, due to the fact that for $Bi^{3+}$ ions, their extended $6s$ orbitals have enhanced hybridization with the O-$2p$ orbitals, leading to significant changes in the band structure comparing to those of the other compounds (cf. Fig. 1). For all the other compounds, the bandwidth and hybridization function are determined by the Ir-O-Ir bond angle and the Ir-O bond length, which are both controlled by $x$. On the one hand, a 180° Ir-O-Ir bond angle would correspond to a situation where two corner sharing $IrO_6$ octahedra have two $IrO_4$ plaquettes on the same plane, favoring electrons hopping between two iridium atoms via the oxygen atoms in between. Bending of the Ir-O-Ir bond leads to smaller hopping parameters of electrons between Ir atoms, and hence smaller Ir-O-Ir bond angle giving rise to a reduced band-width, as shown in Fig. 3. On the other hand, a shorter Ir-O distance can enhance the hybridization between Ir $d$ and O $p$ orbitals, leading to larger hopping and hence larger band-width. This is also true for the rare-earth compounds, as shown in Fig. 3. Therefore, the internal oxygen coordinate is the most important structural parameter, which determines the bandwidth and hence the ground state.

## III. DISTORTED $J = 1/2$ WAVE FUNCTIONS

For all pyrochlore compounds considered in this work, the $IrO_6$ octahedra are compressed along one of the 111 directions. For the one compressed along (111), the resulting trigonal crystal field in the $\{d_{yz}, d_{zx}, d_{xy}\}$ basis can be expressed as

$$H_{\text{trigonal}} = \frac{\delta}{3}\begin{pmatrix} 0 & 1 & 1 \\ 1 & 0 & 1 \\ 1 & 1 & 0 \end{pmatrix}. \quad (1)$$

where $\delta$ denotes the strength of the trigonal crystal-field splitting. We observed that $\delta$ has a significant value, as listed in Table. I. It is comparable to the strength of the atomic SOC of Ir atoms (about 0.5 eV), in good agreement with resonant x-ray scattering measurements.[14] Correspondingly, the $J = 1/2$ wave functions in pyrochlore iridates are strongly distorted, leading to an orbital-to-spin ratio of magnetic moments that deviates significantly from the $SU(2)$ limit (Table I). For instance, in $Y_2Ir_2O_7$ the ratio of orbital to spin moment is about 1.27, which deviates significantly from the ideal value of 2. This can be verified in future experiments using non-resonant magnetic x-ray diffraction, as done for $Sr_2IrO_4$.[15] Furthermore, we observed that the ordered orbital and spin moments are not pointing along the same direction. In our calculations, the total magnetic moments are fixed along the (111) direction following the AIAO pattern, whereas the spin and orbital moments deviate from this direction. The angle between these two moments can be as large as 42° as listed in Table I, which is much larger than that in $Sr_2IrO_4$ (about 5°).

TABLE I: Trigonal crystal field parameter $\delta$, ratio of orbital to spin moments $\mu_L/\mu_S$, and the angle between the orbital and spin moments $\alpha_{LS}$ in $R_2Ir_2O_7$

| | Y | Eu | Sm | Nd | Pr | Bi |
|---|---|---|---|---|---|---|
| $\delta$ (eV) | 0.35 | 0.42 | 0.43 | 0.43 | 0.30 | 0.42 |
| $\mu_L/\mu_S$ | 1.27 | 1.28 | 1.28 | 1.25 | N.A. | N.A. |
| $\alpha_{LS}$ (°) | 31 | 41 | 41 | 42 | N.A. | N.A. |

## IV. EVOLUTION OF THE EIGENVALUES AT THE X POINT

As stated in the main text, at the $X$ point in the Brillouin zone, the fourfold degeneracy is guaranteed by symmetry, with each degenerate group comprising two even-parity and two odd-parity states. Unlike at the $L$ ($L'$) point, where one occupied eigenstate exchanges its parity with one unoccupied eigenstate when the DMFT

self-energies are considered, no band inversion or other change in the ordering of parities between occupied and unoccupied eigenstates occurs at the $X$ point, as shown in Fig. 4. Apparently, each fourfold-degenerate state is split into two doubly degenerate states when the DMFT self energies are considered, due to the breaking of time-reversal symmetry. Therefore, the number of occupied states with odd parities does not change after considering the DMFT self energies, as summarized in Table. I in the Main Text.

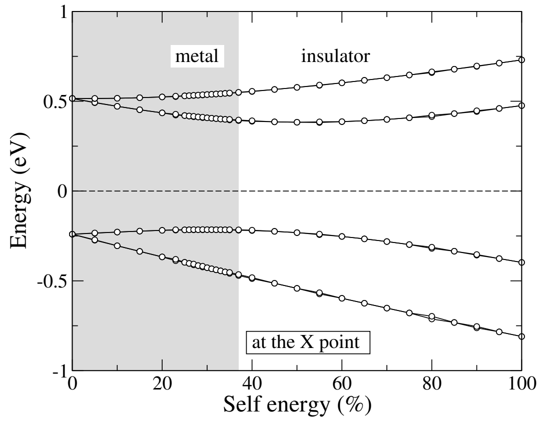


FIG. 4: (Color online) Evolution of the eigenvalues of the effective topological Hamiltonian at $X$ with mixing fraction of the DMFT self-energy. Lines are guides for the eyes.

## V. SPECTRAL FUNCTION WITH SMALLER $U$

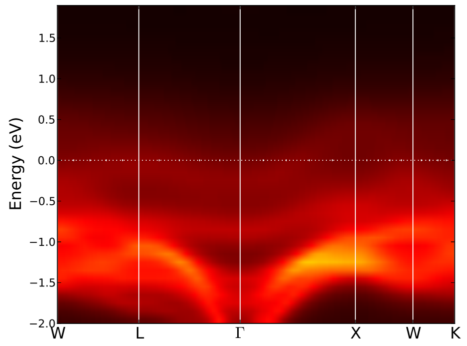


FIG. 5: (Color online) LDA+DMFT spectral function of $Y_2Ir_2O_7$ with on-site $U = 4.0$ eV for Ir atoms.

To check the possibility of achieving topologically a nontrivial semi-metal or axion-insulator phase by reducing the value of the $U$ parameter on the Ir atoms,[16,17] we performed LDA+DMFT calculations for $Y_2Ir_2O_7$ with the on-site $U$ reduced to 4.0 eV. The corresponding spectral function is shown in Fig. 5. In this case, the AIAO magnetic state is not stable and it spontaneously converges to the paramagnetic solution.

* corresp. author: hzhang@physics.rutgers.edu

1 K. Haule, C.-H. Yee, and K. Kim, Phys. Rev. B **81**, 195107 (2010).
2 http://www.wien2k.at
3 K. Haule, Phys. Rev. B **75**, 155113 (2007).
4 J.P. Perdew and Y. Wang, Phys. Rev. B **45**, 13244 (1992).
5 H. Zhang, K. Haule, and D. Vanderbilt, Phys. Rev. Lett. **111**, 246402 (2013).
6 H. Guo, K. Matsuhira, I. Kawasaki, M. Wakeshima, and Y. Hinatsu, Phys. Rev. B **88**, 060411(R) (2013).
7 K. Haule, and T. Birol, arXiv:1501.06936.
8 Y.S. Lee, S.J. Moon, S.C. Riggs, M.C. Shapiro, I.R. Fisher, B.W. Fulfer, J.Y. Chan, A.F. Kemper, and D.N. Basov, Phys. Rev. B **87**, 195143 (2013).
9 J.P. Clancy, *unpublished*
10 J.N. Millican, R.T. Macaluso, S. Nakatsuji, Y. Machida, Y. Maeno, J.Y. Chan, Mat. Res. Bull. **42**, 928 (2007).
11 S.M. Disseler, C. Dhital, T.C. Hogan, A. Amato, S.R. Giblin, C. de la Cruz, A. Daoud-Aladine, S.D. Wilson, and M.J. Graf, Phys. Rev. B **85**, 174441 (2012).
12 K. Matsuhira, M. Wakeshima, R. Nakanishi, T. Yamada, A. Nakamura, W. Kawano, S. Takagi, and Y. Hinatsu, J. Phys. Soc. Jpn. **76**, 043706 (2007).
13 http://www.vasp.at
14 L. Hozoi, H. Gretarsson, J.P. Clancy, B.-G. Jeon, B. Lee, K.H. Kim, V. Yushankhai, P. Fulde, Y.-J. Kim, J. van den Brink, arXiv:1212.4009.
15 S. Fujiyama, H. Ohsumi, K. Ohashi, D. Hirai, B.J. Kim, T. Arima, M. Takata, and H. Takgai, Phys. Rev. Lett. **112**, 016405 (2014).
16 X. Wan, A.M. Turner, A. Vishwanath, and S.Y. Savrasov, Phys. Rev. B **83**, 205101 (2011).
17 A. Go, W. Witczak-Krempa, G.S. Jeon, K. Park, and Y.B. Kim, Phys. Rev. Lett. **109**, 066401 (2012).
